# Supplementary material for: Robust Asymmetric Learning in POMDPs
Source: arXiv:2012.15566 source file (2021-07-01)
Supplement: Supplementary file 1 [file supp_gridworld_a2d.tex]

\begin{figure*}[!htb]

    \begin{subfigure}[t]{0.48\textwidth}
        \includegraphics[width=0.95\textwidth]{figures/sec4/supp/sec4_a2dplot_IceLake_True_MiniGrid-LavaGapS7-v0_arXiv_final_2020_09_01__11_57_59_.pdf}
        \caption{Ice Lake.}
        \label{supp:fig:grid:a2dplot_1:lg}
    \end{subfigure}%
    \hfill%
    \begin{subfigure}[t]{0.48\textwidth}
        \includegraphics[width=0.95\textwidth]{figures/sec4/supp/sec4_a2dplot_TigerDoor_True_MiniGrid-TigerDoorEnv-v0_arXiv_final_2020_09_01__11_57_29_.pdf}
        \caption{Tiger Door.}
        \label{supp:fig:grid:a2dplot_1:td}
    \end{subfigure}%

    \caption{Additional results for the gridworld experiments presented in Figure \ref{fig:gridworld_asym}.  Training curves for the expert and trainee during A2D training, and the projection loss between the expert and trainee.  Due to the annealing effect of $\beta$ we can see that the $\mathbb{KL}$ divergence between expert and trainee (projection loss) rises as the expert learns to solve the MDP, but then reduces to zero as $\beta$ approaches zero and the POMDP is solved instead.  This is particularly pronounced in tiger door, where the performance of the trainee lags behind slightly, as the expert actually optimizes the MDP, initially limiting the performance in the POMDP, before being forced to optimize the POMDP, and then closing the performance gap.  Both expert and trainee converge to the same reward and form an identifiable process pair. 
    }
    \label{supp:fig:grid:a2dplot}
\end{figure*}
